# Supplementary material for: Grasping AI: experiential exercises for designers
Source: arXiv:2310.01282 source file (2023-10-02)
Supplement: Supplementary file 1 [file 06-Appendix.tex]

\newpage
\section{Appendix}
\label{sec:Appendix}

\fig[1.0]{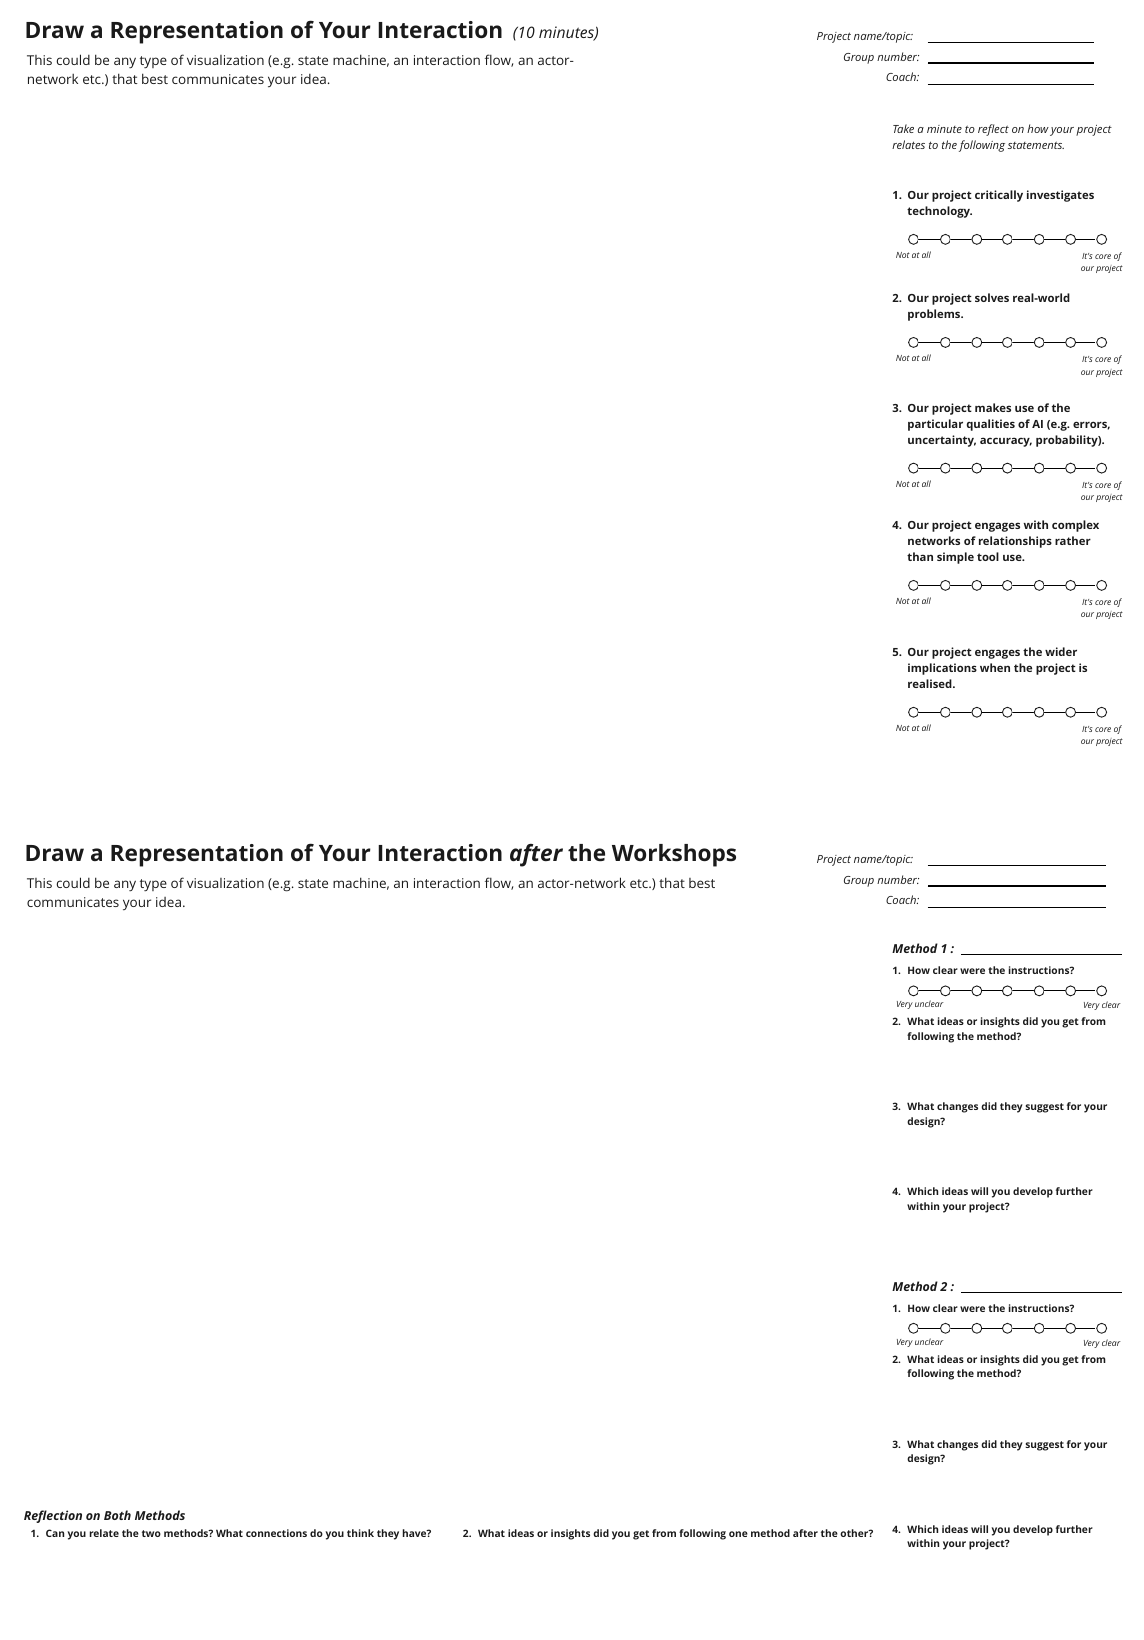}{WORKSHEETS}{A3 Worksheets for the exercise}

\section{Interview Structure and Questions}
\subsection{Questions to Students}

\textbf{About the methods cards (5 mins )}

Why did you select these methods? Can you elaborate on the expectations you had in selecting these?
What did you find useful from these methods ? What was not so useful?
Did you look at the related example projects or literature? If so, was it helpful?
Did you read the background for the method, and was it helpful?
Did you follow the method exactly, or did you adapt/appropriate it to your particular project?
Did one method support the other? Was the ordering important? Were there particular synergies?

\textbf{About the methods in relation to the design concept (5 mins)}

Would you say these methods help you to develop your concept further?  Would you say your concept improved? In which way?
Here is the drawing that you made before and after doing the methods. What would you say are the important differences between them? Was that due to a particular thing that happened through doing a method?
What was the feeling of the group after using these methods? Would you say the group feels now more equiped in designing with AI in your project after the workshop?

\textbf{About  AI qualities  as a design resource (around 3 mins per section)}

\textbf{Affordances:}
What aspects or qualities of AI became more apparent present that you were not considering before?
Some methods asked you to role-play AI, or draw a diagram of the system. Do you think this way of engaging with AI helped to understand AI in a different way? Why?

\textbf{Relations:}
Do you think the workshop helped you with considering AI as something other than just a tool?
Did the methods help you consider the AI in your project as part of a broader network of relationships? What new relations did it uncover?

\textbf{Wider implications:}
Did the methods make you think more critically about the possible broader implications and challenges of your project?  In which way?
Did the methods help you to consider how interactions might change over time?

\textbf{Final reflections (5 mins)}

Overall, did the workshop contribute to developing a new understanding of designing with and for AI?
Have you thought about using another of the methods in your own process?
Do you have any final reflection or questions?

\subsection{Questions for coaches}

\textbf{Warm up: }
How are your students/ teams progressing in the course? What can you say about their general understanding of designing with/ for AI?
How comprehensive do you feel is your understanding of AI and its use in design?
Did you have previous research/practice experience with AI and design?

\textbf{Consider for each group: }
How much did you discuss AI with them, as opposed to general interactive prototyping? Was there a significant engagement with AI in the coach meetings?
If you look at the work before and after the workshop, did you feel that the methods workshop helped the students? In what way?
Did the students engage with the particular qualities of AI (e.g. uncertainty, training, data use) a) before the workshop, b) after the workshop?
Did the students think about their project as a tool, or as part of a wider network of relations a) before the workshop, b) after the workshop
Did the students think critically about the implications of their project (social shaping, change over time, privacy etc.) a) before the workshop, b) after the workshop
Did you notice  changes  due to any particular  method reflected in the progress and development of any of the student challenges?
